# Supplementary material for: Adnexal Mass Segmentation with Ultrasound Data Synthesis
Source: arXiv:2209.12305 source file (2022-09-25)
Supplement: Supplementary file 1 [file appendix.tex]

\appendix
\section{Appendix}

\begin{table}[htp]
\centering
\resizebox{\textwidth}{!}{%
\begin{tabular}{@{}p{1cm}p{4cm}p{4cm}p{4cm}p{4cm}@{}}
\toprule
\multicolumn{1}{l}{\textbf{Machine}} & \multicolumn{1}{l}{\textbf{1}}            & \multicolumn{1}{l}{\textbf{2}}           & \textbf{3}                       & \textbf{4}                                \\ \midrule
\textbf{GPU}                                  & GM200 {[}GeForce GTX TITAN X{]}           & GA102GL {[}RTX A6000{]}                  & GA102GL {[}RTX A5000{]}          & GA102 {[}GeForce RTX 3090{]}              \\
\textbf{CPU}                                  & Intel(R) Xeon(R) CPU E5-1630 v3 @ 3.70GHz & Intel(R) Xeon(R) Gold 6230 CPU @ 2.10GHz & AMD EPYC 7502P 32-Core Processor & Intel(R) Core(TM) i9-10920X CPU @ 3.50GHz \\
\textbf{RAM}                                  & 66GB                                      & 192GB                                    & 258GB                            & 130GB                                     \\ \bottomrule
\end{tabular}%
}
\caption{Specification of machines used to carry out our experiments}
\label{machines_used}
\end{table}
